# Supplementary material for: A Uniqueness Theorem for Incompressible Fluid Flows with Straight Streamlines
Source: arXiv:2201.02862 source file (2022-01-08)
Supplement: Supplementary file 1 [file Appendix_to__Incompressible_Fluid_Flows_with_Straight_Streamlines_.pdf]

# A UNIQUENESS THEOREM FOR INCOMPRESSIBLE FLUID FLOWS WITH STRAIGHT STREAMLINES

BRENDAN GUILFOYLE

ABSTRACT. These Appendices contain REDUCE computer algebra code [1] for the computations behind Propositions 3.1, 3.2 and 3.3, as well as Theorems 4.1, 4.2, 5.1, 5.2 and 6.1 of the above paper.

In particular the rank two proofs are in Appendix A, the rank one proofs in Appendix B and the rank zero proofs Appendix C.

## APPENDIX A. RANK TWO STRAIGHT STREAMLINES

The following code contains the calculations needed for the proof of the rank two divergence-free condition in Proposition 3.1 and the steady case of the Main Theorem for rank two line congruences, namely Theorem 4.1.

```
%*********************************************************
% Rank Two Euler Flows with Straight Streamlines
%  Prop 3.1 and Thm 4.1
%*********************************************************
% Steady
%******************************
% Congruence coordinates
on gcd$ depend eta,xi,xib$ depend etab,xi,xib$
z:=2*(eta-xi**2*etab)/(1+xi*xib)**2+2*xi*r/(1+xi*xib)$
zb:=2*(etab-xib**2*eta)/(1+xi*xib)**2+2*xib*r/(1+xi*xib)$
x3:=-2*(xib*eta+xi*etab)/(1+xi*xib)**2+(1-xi*xib)*r/(1+xi*xib)$

% Compute pulled back metric and inverse
array gdd(2,2),gnewdd(2,2),x(2),y(2),vu(2)$
y(0):=z$ y(1):=zb$ y(2):=x3$  x(0):=xi$ x(1):=xib$ x(2):=r$
gnewdd(0,1):=1/2$ gnewdd(1,0):=1/2$ gnewdd(2,2):=1$
for ii:=0:2 do for jj:=0:2 do
  gdd(ii,jj):=for kk:=0:2 sum for ll:=0:2 sum
    gnewdd(kk,ll)*df(y(kk),x(ii))*df(y(ll),x(jj))$
array guu(2,2)$ matrix matgdd(3,3), matguu(3,3)$
for ii:=0:2 do for jj:=ii:2 do matgdd(ii+1,jj+1):=gdd(ii,jj)$
for ii:=0:2 do for jj:=ii:2 do matgdd(jj+1,ii+1):= matgdd(ii+1,jj+1)$
matguu := 1/matgdd$
for ii:=0:2 do for jj:=ii:2 do guu(ii,jj):= matguu(ii+1,jj+1)$
for ii:=0:2 do for jj:=ii:2 do guu(jj,ii) :=guu(ii,jj)$
```

*Date*: January 8, 2022.

```
clear matgdd, matguu$

% Compute Christoffel symbols of 1st and 2nd kind
array chrisddd(2,2,2),chrisddu(2,2,2)$
for ii:=0:2 do for jj:=ii:2 do  <<for kk:=0:2 do chrisddd(jj,ii,kk)
   := chrisddd(ii,jj,kk):= (df(gdd(jj,kk),x(ii))
   +df(gdd(kk,ii),x(jj))-df(gdd(ii,jj),x(kk)))/2$
for kk:=0:2 do chrisddu(jj,ii,kk):= chrisddu(ii,jj,kk)
   := for pp := 0:2 sum guu(kk,pp)*chrisddd(ii,jj,pp) >>$

% Replace derivatives of F by sigma, lambda, theta
depend sig,xi,xib$ depend sigb,xi,xib$ depend lam,xi,xib$ depend tta,xi,xib$
let df(etab,xi)=-sig$ let df(eta,xib)=-sigb$
let df(eta,xi)=2*xib*eta/(1+xi*xib)+tta+i*lam$
let df(etab,xib)=2*xi*etab/(1+xi*xib)+tta-i*lam$

% Velocity Vector Field
Vu(2):=Vr$ depend Vr,r,xi,xib$

% Compute the divergence
adiv:=for ii:=0:2 sum for jj:=0:2 sum chrisddu(ii,jj,ii)*Vu(jj)$
bdiv:=for ii:=0:2 sum df(Vu(ii),x(ii))$ div:=adiv+bdiv$

%The divergence-free condition Prop 3.1
depend h,xi,xib$ VR:=H/(r**2+r*(1+xi*xib)**2*(df(eta/(1+xi*xib)**2,xi)
   +df(etab/(1+xi*xib)**2,xib))+(1+xi*xib)**4*df(eta/(1+xi*xib)**2,xi)
   *df(etab/(1+xi*xib)**2,xib)-df(etab,xi)*df(eta,xib))$
div:=div;

%Euler equations Thm 4.1
array tens4u(2),tens5u(2),convu(2),euleru(2),dpu(2)$ depend p,xi,xib,r$
for ii:=0:2 do tens4u(ii):=for jj:=0:2 sum Vu(jj)*df(Vu(ii),x(jj))$
for ii:=0:2 do tens5u(ii):=
   for jj:=0:2 sum for kk:=0:2 sum Vu(jj)*Vu(kk)*chrisddu(jj,kk,ii)$
for ii:=0:2 do convu(ii):=tens4u(ii)+tens5u(ii)$
for ii:=0:2 do dpu(ii):=for jj:=0:2 sum guu(ii,jj)*df(p,x(jj))$
for ii:=0:2 do euleru(ii):=-convu(ii)-dpu(ii)$

% Solutions
let df(p,xi)=-2*df(p,r)*etab/(1+xi*xib)**2$
let df(p,xib)=-2*df(p,r)*eta/(1+xi*xib)**2$ euleru(0); euleru(1);
let df(p,r)=2*(r+tta)*H**2/((r+tta)**2+lam**2-sig*sigb)**3$ euleru(2);

%*****************************

% Substituting Solutions back in Eqn (10)
on gcd$
depend k,xi,xib$ depend h,xi,xib$ depend sig,xi,xib$ depend sigb,xi,xib$
```

```
depend lam,xi,xib$ depend tta,xi,xib$
 p:=K-h**2/(2*(lam**2+(r+tta)**2-sig*sigb)**2)$
test1:=df(p,r)-2*(r+tta)*H**2/((r+tta)**2+lam**2-sig*sigb)**3;
eqn1:=num(df(p,xi)+2*df(p,r)*etab/(1+xi*xib)**2)$
eqn1a:=df(eqn1,r,6); k:=p0$ eqn1a;
eqn1b:=df(eqn1,r,2); h:=h0$ eqn1b;
eqn1c:=df(eqn1,r); let df(tta,xi)=-2*etab/(1+xi*xib)**2$
let df(tta,xib)=-2*eta/(1+xi*xib)**2$ eqn1c;
lam:=0$ eqn12:=-num(eqn1)/(h0**2*(1+xi*xib)**2);
sig:=0$ sigb:=0$
eqn1;
```

The next code contains the calculations needed for the proof of Theorem 4.2 for rank two non-steady flows. This has three cases (i), (ii) and (iii). Only case (ii) yields solutions.

```
%**********************************************************
% Rank Two Euler Flows with Straight Streamlines
%  Thm 4.2
%**********************************************************
% Non-Steady
%*****************************
% Congruence coordinates
on gcd$ depend eta,xi,xib$ depend etab,xi,xib$
z:=2*(eta-xi**2*etab)/(1+xi*xib)**2+2*xi*r/(1+xi*xib)$
zb:=2*(etab-xib**2*eta)/(1+xi*xib)**2+2*xib*r/(1+xi*xib)$
x3:=-2*(xib*eta+xi*etab)/(1+xi*xib)**2+(1-xi*xib)*r/(1+xi*xib)$

% Compute pulled back metric and inverse
array gdd(2,2),gnewdd(2,2),x(2),y(2),vu(2)$
y(0):=z$ y(1):=zb$ y(2):=x3$  x(0):=xi$ x(1):=xib$ x(2):=r$
gnewdd(0,1):=1/2$ gnewdd(1,0):=1/2$ gnewdd(2,2):=1$
for ii:=0:2 do for jj:=0:2 do
  gdd(ii,jj):=for kk:=0:2 sum for ll:=0:2 sum
    gnewdd(kk,ll)*df(y(kk),x(ii))*df(y(ll),x(jj))$
array guu(2,2)$ matrix matgdd(3,3), matguu(3,3)$
for ii:=0:2 do for jj:=ii:2 do matgdd(ii+1,jj+1):=gdd(ii,jj)$
for ii:=0:2 do for jj:=ii:2 do matgdd(jj+1,ii+1):= matgdd(ii+1,jj+1)$
matguu := 1/matgdd$
for ii:=0:2 do for jj:=ii:2 do guu(ii,jj):= matguu(ii+1,jj+1)$
for ii:=0:2 do for jj:=ii:2 do guu(jj,ii) :=guu(ii,jj)$
clear matgdd, matguu$

% Compute Christoffel symbols of 1st and 2nd kind
array chrisddd(2,2,2),chrisddu(2,2,2)$
for ii:=0:2 do for jj:=ii:2 do  <<for kk:=0:2 do chrisddd(jj,ii,kk)
   := chrisddd(ii,jj,kk):= (df(gdd(jj,kk),x(ii))+df(gdd(kk,ii),x(jj))
    -df(gdd(ii,jj),x(kk)))/2$
for kk:=0:2 do chrisddu(jj,ii,kk):= chrisddu(ii,jj,kk)
```

```
   := for pp := 0:2 sum guu(kk,pp)*chrisddd(ii,jj,pp) >>$

% Substitute derivatives of F for sigma, lambda, theta
depend sig,xi,xib$ depend sigb,xi,xib$ depend lam,xi,xib$ depend tta,xi,xib$
let df(etab,xi)=-sig$ let df(eta,xib)=-sigb$
let df(eta,xi)=2*xib*eta/(1+xi*xib)+tta+i*lam$
let df(etab,xib)=2*xi*etab/(1+xi*xib)+tta-i*lam$

% Velocity vector field
Vu(2):=Vr$ depend Vr,r,xi,xib,t$

% Compute the divergence
adiv:=for ii:=0:2 sum for jj:=0:2 sum chrisddu(ii,jj,ii)*Vu(jj)$
bdiv:=for ii:=0:2 sum df(Vu(ii),x(ii))$
div:=adiv+bdiv$

% The divergence-free condition Prop 3.1
depend h,xi,xib,t$ VR:=H/(r**2+r*(1+xi*xib)**2*(df(eta/(1+xi*xib)**2,xi)
  +df(etab/(1+xi*xib)**2,xib))+(1+xi*xib)**4*df(eta/(1+xi*xib)**2,xi)
  *df(etab/(1+xi*xib)**2,xib)-df(etab,xi)*df(eta,xib))$
div:=div;

% Euler equations
array tens4u(2),tens5u(2),convu(2),euleru(2),dpu(2)$ depend p,xi,xib,r$
for ii:=0:2 do tens4u(ii):=for jj:=0:2 sum Vu(jj)*df(Vu(ii),x(jj))$
for ii:=0:2 do tens5u(ii):=
   for jj:=0:2 sum for kk:=0:2 sum Vu(jj)*Vu(kk)*chrisddu(jj,kk,ii)$
for ii:=0:2 do convu(ii):=tens4u(ii)+tens5u(ii)$
for ii:=0:2 do dpu(ii):=for jj:=0:2 sum guu(ii,jj)*df(p,x(jj))$
for ii:=0:2 do euleru(ii):=-df(vu(ii),t)-convu(ii)-dpu(ii)$

% Proof of Thm 4.2
let df(p,xi)=-2*df(p,r)*etab/(1+xi*xib)**2$
let df(p,xib)=-2*df(p,r)*eta/(1+xi*xib)**2$ euleru(0); euleru(1);
let df(p,r)=2*(r+tta)*H**2/((r+tta)**2+lam**2-sig*sigb)**3
  -df(h,t)/((r+tta)**2+lam**2-sig*sigb)$ euleru(2);

%*****************************
% Thm 4.2 Case (i)
%*****************************
on gcd$
depend k,xi,xib,t$ depend h,xi,xib,t$ depend sig,xi,xib$ depend sigb,xi,xib$
depend lam,xi,xib$ depend tta,xi,xib$ depend gam,xi,xib,r$
p:=K-h**2/(2*(lam**2+(r+tta)**2-sig*sigb)**2)-df(h,t)*gam/sqrt(lam**2-sig*sigb)$
depend gam,xi,xib,r$ let df(gam,r)=df(atan((r+tta)/sqrt(lam**2-sig*sigb)),r)$
let df(gam,xi)=df(atan((r+tta)/sqrt(lam**2-sig*sigb)),xi)$
let df(gam,xib)=df(atan((r+tta)/sqrt(lam**2-sig*sigb)),xib)$
test1:=df(p,r)-2*(r+tta)*H**2/((r+tta)**2+lam**2-sig*sigb)**3
```

```
   +df(h,t)/((r+tta)**2+lam**2-sig*sigb);

% Substituting Solutions back in Eqn (12)
ans1:=num(df(p,xi)+2*df(p,r)*etab/(1+xi*xib)**2)$
al:=(limit(num(ans1),gam,0))$ be:=(df(num(ans1),gam))$
ans4:=(df(al,r,6)); k:=k0$ ans4;
ans5:=(df(be,r,6));  let df(h,t)=Aa*sqrt(lam**2-sig*sigb)$ depend aa,t$ ans5;
ans6:=(df(al,r,5)); let df(lam,xi)=(sig*df(sigb,xi)+sigb*df(sig,xi))/(2*lam)$
let df(lam,xib)=(sig*df(sigb,xib)+sigb*df(sig,xib))/(2*lam)$ ans6;
ans7:=(df(al,r,4)); let df(tta,xi)=-2*etab/(1+xi*xib)**2$
let df(tta,xib)=-2*eta/(1+xi*xib)**2$ ans7;

%******************************
% Thm 4.2 Case (ii)
%******************************
on gcd$
depend k,xi,xib,t$ depend h,xi,xib,t$ depend hd,xi,xib$ depend sig,xi,xib$
depend sigb,xi,xib$ depend lam,xi,xib$ depend tta,xi,xib$
p:=K-h**2/(2*(r+tta)**4)+df(h,t)/(r+tta)$
test1:=df(p,r)-2*(r+tta)*H**2/((r+tta)**2)**3+df(h,t)/((r+tta)**2);

% Substituting Solutions back in Eqn (12)
ans1:=num(df(p,xi)+2*df(p,r)*etab/(1+xi*xib)**2)$
ans2:=(df(num(ans1),r,5)); k:=k0$ ans2;
ans3:=(df(num(ans1),r,4)); let df(h,t)=h0d$ ans3;
ans4:=(df(num(ans1),r,3));  let df(tta,xi)=-2*etab/(1+xi*xib)**2$
let df(tta,xib)=-2*eta/(1+xi*xib)**2$ ans4;
ans5:=df(num(ans1),r);  h:=h0$ ans5;

%******************************
% Thm 4.2 Case (iii)
%******************************
on gcd$
depend k,xi,xib,t$ depend h,xi,xib,t$ depend sig,xi,xib$ depend sigb,xi,xib$
depend lam,xi,xib$ depend tta,xi,xib$
p:=K-h**2/(2*(lam**2+(r+tta)**2-sig*sigb)**2)
-df(h,t)*gam/(2*sqrt(sig*sigb-lam**2))$ depend gam,xi,xib,r$
let df(gam,r)=df(log((r+tta-sqrt(sig*sigb-lam**2))/(r+tta+sqrt(sig*sigb-lam**2))),r)$
let df(gam,xi)=df(log((r+tta-sqrt(sig*sigb-lam**2))/(r+tta+sqrt(sig*sigb-lam**2))),xi)$
let df(gam,xib)=df(log((r+tta-sqrt(sig*sigb-lam**2))/(r+tta+sqrt(sig*sigb-lam**2))),xib)$
test1:=df(p,r)-2*(r+tta)*H**2/((r+tta)**2+lam**2-sig*sigb)**3
   +df(h,t)/((r+tta)**2+lam**2-sig*sigb);

% Substituting solutions back in Eqn (12)
ans1:=num(df(p,xi)+2*df(p,r)*etab/(1+xi*xib)**2)$
al:=(limit(num(ans1),gam,0))$ be:=(df(num(ans1),gam))$
ans4:=(df(al,r,6)); k:=k0; ans4;
ans5:=(df(be,r,6));  let df(h,t)=A*sqrt(sig*sigb-lam**2)$ ans5;
```

```
ans6:=(df(al,r,5)); let df(lam,xi)=(sig*df(sigb,xi)+sigb*df(sig,xi))/(2*lam)$
let df(lam,xib)=(sig*df(sigb,xib)+sigb*df(sig,xib))/(2*lam)$ ans6;
ans7:=(df(al,r,4)); let df(tta,xi)=-2*etab/(1+xi*xib)**2$
let df(tta,xib)=-2*eta/(1+xi*xib)**2$  ans7;
lam:=0$ sig:=0$ sigb:=0$
ans8:=(df(al,r,2)); h:=h0$ ans8;
ans9:=(df(al,r)); eta:=0$ etab:=0$ ans9;
```

## Appendix B. Rank One Straight Streamlines

The following code contains the calculations needed for the proof of the rank one divergence-free condition in Proposition 3.2 and the Main Theorem for steady rank one flows, namely Theorem 5.1.

```
%***********************************************************
% Rank One Euler Flows with Straight Streamlines
%  Prop 3.2 and Thm 5.1
%***********************************************************
% Steady
%*****************************
% Congruence coordinates
on gcd$
depend xi,u$ depend xib,u$  depend eta,u,v$ depend etab,u,v$
z:=2*(eta-xi**2*etab)/(1+xi*xib)**2+2*xi*r/(1+xi*xib)$
zb:=2*(etab-xib**2*eta)/(1+xi*xib)**2+2*xib*r/(1+xi*xib)$
t:=-2*(xib*eta+xi*etab)/(1+xi*xib)**2+(1-xi*xib)*r/(1+xi*xib)$

% Compute pulled back metric and inverse
array gdd(2,2),gnewdd(2,2),x(2),y(2),vu(2)$
y(0):=z$ y(1):=zb$ y(2):=t$  x(0):=u$ x(1):=v$ x(2):=r$
gnewdd(0,1):=1/2$ gnewdd(1,0):=1/2$ gnewdd(2,2):=1$
for ii:=0:2 do for jj:=0:2 do
gdd(ii,jj):=for kk:=0:2 sum for ll:=0:2 sum gnewdd(kk,ll)*df(y(kk),x(ii))*df(y(ll),x(jj))$
array guu(2,2)$ matrix matgdd(3,3), matguu(3,3)$
for ii:=0:2 do for jj:=ii:2 do matgdd(ii+1,jj+1):=gdd(ii,jj)$
for ii:=0:2 do for jj:=ii:2 do matgdd(jj+1,ii+1):= matgdd(ii+1,jj+1)$
matguu := 1/matgdd$
for ii:=0:2 do for jj:=ii:2 do guu(ii,jj):= matguu(ii+1,jj+1)$
for ii:=0:2 do for jj:=ii:2 do guu(jj,ii) :=guu(ii,jj)$
clear matgdd, matguu$

% Compute Christoffel symbols of 1st and 2nd kind
array chrisddd(2,2,2),chrisddu(2,2,2)$
for ii:=0:2 do for jj:=ii:2 do  <<for kk:=0:2 do chrisddd(jj,ii,kk)
  := chrisddd(ii,jj,kk):= (df(gdd(jj,kk),x(ii))+df(gdd(kk,ii),x(jj))
  -df(gdd(ii,jj),x(kk)))/2$
for kk:=0:2 do chrisddu(jj,ii,kk):= chrisddu(ii,jj,kk) :=
   for pp := 0:2 sum guu(kk,pp)*chrisddd(ii,jj,pp) >>$
```

```
% Velocity Vector Field
Vu(2):=Vr$ depend Vr,u,v,r$

% Compute the divergence
adiv:=for ii:=0:2 sum for jj:=0:2 sum chrisddu(ii,jj,ii)*Vu(jj)$
bdiv:=for ii:=0:2 sum df(Vu(ii),x(ii))$
div:=adiv+bdiv$

% The divergence-free condition Prop 3.2
depend h,u,v$ aa:=-(df(eta,v)*df(xib,u)-df(etab,v)*df(xi,u))*(1+xi*xib)$
bb:=(df(etab,v)*df(eta,u)-df(eta,v)*df(etab,u))*(1+xi*xib)
   +2*(etab*xi*df(xib,u)*df(eta,v)-eta*xib*df(xi,u)*df(etab,v))$
VR:=h/(r+bb/aa)$ div:=div;

% Euler equations
array tens4u(2),tens5u(2),convu(2),euleru(2),dpu(2)$ depend p,u,v,r$
for ii:=0:2 do tens4u(ii):=for jj:=0:2 sum Vu(jj)*df(Vu(ii),x(jj))$
for ii:=0:2 do tens5u(ii):=
  for jj:=0:2 sum for kk:=0:2 sum Vu(jj)*Vu(kk)*chrisddu(jj,kk,ii)$
for ii:=0:2 do convu(ii):=tens4u(ii)+tens5u(ii)$
for ii:=0:2 do dpu(ii):=for jj:=0:2 sum guu(ii,jj)*df(p,x(jj))$
for ii:=0:2 do euleru(ii):=-convu(ii)-dpu(ii)$

% Proof of Thm 5.1
p:=p00-h**2/(2*(r+be)**2)$ depend be,u$  depend p00,u$ let df(h,v)=0$
ans1:=df(num(euleru(0)),r,3); let df(p00,u)=0$ ans1;
ans2:=df(num(euleru(0)),r); let df(h,u)=0$ ans2;
depend L,v$ eta:=(-(1+xi*xib)**2*df(be,u)/(4*df(xi,u)*df(xib,u))+i*l)*df(xi,u)$
etab:=(-(1+xi*xib)**2*df(be,u)/(4*df(xi,u)*df(xib,u))-i*l)*df(xib,u)$
euleru(0); euleru(1);

% Polar coordinates
depend rr,u$ depend phi,u$ xi:=rr*e**(i*phi)$ xib:=rr*e**(-i*phi)$ phi:=0$ rr:=u$
be:=(b0*(1-u**2)+2*b1*u)/(1+u**2)$
euleru(0); euleru(1); euleru(2);
Vr;
p-p00;
xi;
eta;
```

The following code contains the calculations needed for the proof of the Main Theorem for non-steady rank one flows, namely Theorem 5.2.

```
%**********************************************************
% Rank One Euler Flows with Straight Streamlines
%   Thm 5.2
%**********************************************************
% Non-Steady Case
```

```
%*****************************
% Congruence coordinates
on gcd$
depend xi,u$ depend xib,u$  depend eta,u,v$ depend etab,u,v$
z:=2*(eta-xi**2*etab)/(1+xi*xib)**2+2*xi*r/(1+xi*xib)$
zb:=2*(etab-xib**2*eta)/(1+xi*xib)**2+2*xib*r/(1+xi*xib)$
x3:=-2*(xib*eta+xi*etab)/(1+xi*xib)**2+(1-xi*xib)*r/(1+xi*xib)$

% Compute pulled back metric and inverse
array gdd(2,2),gnewdd(2,2),x(2),y(2),vu(2)$
y(0):=z$ y(1):=zb$ y(2):=x3$  x(0):=u$ x(1):=v$ x(2):=r$
gnewdd(0,1):=1/2$ gnewdd(1,0):=1/2$ gnewdd(2,2):=1$
for ii:=0:2 do for jj:=0:2 do
gdd(ii,jj):=for kk:=0:2 sum for ll:=0:2 sum gnewdd(kk,ll)*df(y(kk),x(ii))*df(y(ll),x(jj))$
array guu(2,2)$ matrix matgdd(3,3), matguu(3,3)$
for ii:=0:2 do for jj:=ii:2 do matgdd(ii+1,jj+1):=gdd(ii,jj)$
for ii:=0:2 do for jj:=ii:2 do matgdd(jj+1,ii+1):= matgdd(ii+1,jj+1)$
matguu := 1/matgdd$
for ii:=0:2 do for jj:=ii:2 do guu(ii,jj):= matguu(ii+1,jj+1)$
for ii:=0:2 do for jj:=ii:2 do guu(jj,ii) :=guu(ii,jj)$
clear matgdd, matguu$

% Compute Christoffel symbols of 1st and 2nd kind
array chrisddd(2,2,2),chrisddu(2,2,2)$
for ii:=0:2 do for jj:=ii:2 do  <<for kk:=0:2 do chrisddd(jj,ii,kk)
   := chrisddd(ii,jj,kk):= (df(gdd(jj,kk),x(ii))+df(gdd(kk,ii),x(jj))
    -df(gdd(ii,jj),x(kk)))/2$
for kk:=0:2 do chrisddu(jj,ii,kk):= chrisddu(ii,jj,kk) :=
   for pp := 0:2 sum guu(kk,pp)*chrisddd(ii,jj,pp) >>$

% Velocity Vector Field
Vu(2):=vr$ depend vr,u,v,r,t$

% Compute the divergence
adiv:=for ii:=0:2 sum for jj:=0:2 sum chrisddu(ii,jj,ii)*Vu(jj)$
bdiv:=for ii:=0:2 sum df(Vu(ii),x(ii))$
div:=adiv+bdiv$

% The divergence-free condition Prop 3.2
depend h,u,v$ aa:=-(df(eta,v)*df(xib,u)-df(etab,v)*df(xi,u))*(1+xi*xib)$
bb:=(df(etab,v)*df(eta,u)-df(eta,v)*df(etab,u))*(1+xi*xib)
   +2*(etab*xi*df(xib,u)*df(eta,v)-eta*xib*df(xi,u)*df(etab,v))$
Vr:=h/(r+be)$ depend be,u$ test1:=limit(div,be,bb/aa);

% Euler equations
array tens4u(2),tens5u(2),convu(2),euleru(2),dpu(2)$ depend p,u,v,r$
for ii:=0:2 do tens4u(ii):=for jj:=0:2 sum Vu(jj)*df(Vu(ii),x(jj))$
for ii:=0:2 do tens5u(ii)
```

```
:=for jj:=0:2 sum for kk:=0:2 sum Vu(jj)*Vu(kk)*chrisddu(jj,kk,ii)$
for ii:=0:2 do convu(ii):=tens4u(ii)+tens5u(ii)$
for ii:=0:2 do dpu(ii):=for jj:=0:2 sum guu(ii,jj)*df(p,x(jj))$
for ii:=0:2 do euleru(ii):=-df(Vu(ii),t)-convu(ii)-dpu(ii)$

% Proof of Thm 5.2
let df(p,v)=0$ depend p0,u$ p:=p0-h**2/(2*(r+be)**2)-df(h,t)*log(r+be)$
test2:=-df(p,r)+h**2/(r+be)**3-df(h,t)/(r+be);
eqn1:=num(df(p,u)+2*df(p,r)*(etab*df(xi,u)+eta*df(xib,u))/(1+xi*xib)**2);
ans1:=df(eqn1,log(r+be)); let df(H,t)=hd0$ ans1;
ans2:=df(eqn1,r,3); p0:=p00$ ans2;
ans3:=df(eqn1,r)$ h:=h0$ ans3;
eqn1; depend L,v$ eta:=(-(1+xi*xib)**2*df(be,u)/(4*df(xi,u)*df(xib,u))+i*l)*df(xi,u)$
etab:=(-(1+xi*xib)**2*df(be,u)/(4*df(xi,u)*df(xib,u))-i*l)*df(xib,u)$ eqn1;
euleru(0); euleru(1); euleru(2);

% Polar coordinates
xi:=u$ xib:=u$ be:=(b0*(1-u**2)+2*b1*u)/(1+u**2)$
euleru(0); euleru(1); euleru(2); div;
vr;
p-p00;
xi;
eta;
```

## Appendix C. Rank Zero Straight Streamlines

The following code contains the calculations needed for the proof of the rank zero divergence-free condition in Proposition 3.3 and the Main Theorem for steady rank zero flows, namely Theorem 6.1.

```
%*********************************************************
% Rank Zero Euler Flows with Straight Streamlines
%  Prop 3.3 and Thm 6.1
%*********************************************************
% Congruence coordinates
on gcd$
depend eta,u,v$ depend etab,u,v$
z:=2*(eta-xi**2*etab)/(1+xi*xib)**2+2*xi*r/(1+xi*xib)$
zb:=2*(etab-xib**2*eta)/(1+xi*xib)**2+2*xib*r/(1+xi*xib)$
x3:=-2*(xib*eta+xi*etab)/(1+xi*xib)**2+(1-xi*xib)*r/(1+xi*xib)$

% Compute pulled back metric and inverse
array gdd(2,2),gnewdd(2,2),x(2),y(2),vu(2)$
y(0):=z$ y(1):=zb$ y(2):=x3$  x(0):=u$ x(1):=v$ x(2):=r$
gnewdd(0,1):=1/2$ gnewdd(1,0):=1/2$ gnewdd(2,2):=1$
for ii:=0:2 do for jj:=0:2 do gdd(ii,jj):=
   for kk:=0:2 sum for ll:=0:2 sum gnewdd(kk,ll)*df(y(kk),x(ii))*df(y(ll),x(jj))$
array guu(2,2)$ matrix matgdd(3,3), matguu(3,3)$
```

```
for ii:=0:2 do for jj:=ii:2 do matgdd(ii+1,jj+1):=gdd(ii,jj)$
for ii:=0:2 do for jj:=ii:2 do matgdd(jj+1,ii+1):= matgdd(ii+1,jj+1)$
matguu := 1/matgdd$
for ii:=0:2 do for jj:=ii:2 do guu(ii,jj):= matguu(ii+1,jj+1)$
for ii:=0:2 do for jj:=ii:2 do guu(jj,ii) :=guu(ii,jj)$
clear matgdd, matguu$

% Compute Christoffel symbols of 1st and 2nd kind
array chrisddd(2,2,2),chrisddu(2,2,2)$
for ii:=0:2 do for jj:=ii:2 do  <<for kk:=0:2 do chrisddd(jj,ii,kk)
   := chrisddd(ii,jj,kk):= (df(gdd(jj,kk),x(ii))+df(gdd(kk,ii),x(jj))
    -df(gdd(ii,jj),x(kk)))/2$
for kk:=0:2 do chrisddu(jj,ii,kk):= chrisddu(ii,jj,kk) :=
for pp := 0:2 sum guu(kk,pp)*chrisddd(ii,jj,pp) >>$

% Velocity Vector Field
Vu(2):=vr$ depend vr,u,v,r,t$

% Compute the divergence
adiv:=for ii:=0:2 sum for jj:=0:2 sum chrisddu(ii,jj,ii)*Vu(jj)$
bdiv:=for ii:=0:2 sum df(Vu(ii),x(ii))$
div:=adiv+bdiv$ ans:=num(div)$
div:=div$

% The divergence-free condition Prop 3.3
VR:=H$ depend h,u,v,t$ div:=div;

% Oriented normals to horizontal plane
xi:=0$ xib:=0$ eta:=u+i*v$  etab:=u-i*v$

% Euler equations
array tens4u(2),tens5u(2),convu(2),euleru(2),dpu(2)$ depend p,u,v,r$
for ii:=0:2 do tens4u(ii):=for jj:=0:2 sum Vu(jj)*df(Vu(ii),x(jj))$
for ii:=0:2 do tens5u(ii):=
   for jj:=0:2 sum for kk:=0:2 sum Vu(jj)*Vu(kk)*chrisddu(jj,kk,ii)$
for ii:=0:2 do convu(ii):=tens4u(ii)+tens5u(ii)$
for ii:=0:2 do dpu(ii):=for jj:=0:2 sum guu(ii,jj)*df(p,x(jj))$
for ii:=0:2 do euleru(ii):=-df(Vu(ii),t)-convu(ii)-dpu(ii)$
for ii:=0:2 do dpu(ii):=for jj:=0:2 sum guu(ii,jj)*df(p,x(jj))$
for ii:=0:2 do euleru(ii):=-df(Vu(ii),t)-convu(ii)-dpu(ii)$

% Proof of Thm 6.1
p:=p0-df(h,t)*r$ H:=al+k$ depend al,t$ depend k,u,v$

euleru(0); euleru(1); euleru(2); div;
```

## References

[1] A.C. Hearn, *REDUCE—A case study in algebra system development*, European Computer Algebra Conference, Springer, Berlin, Heidelberg, 1982.

Brendan Guilfoyle, School of STEM, Munster Technological University, Tralee, Co. Kerry, Ireland.
*Email address*: brendan.guilfoyle@mtu.ie
